# Supplementary material for: Object Discovery in Videos as Foreground Motion Clustering
Source: arXiv:1812.02772 source file (2019-04-05)
Supplement: Supplementary file 1 [file appendix.tex]

\appendix

%\section{Y-Net Architecture Details}

\section{PT-RNN Variants}

The three PT-RNN variants to compute the weight $\bb{w}_t$, \textit{standard}, \textit{conv}, and \textit{convGRU} are shown in detail in Table \ref{table:pt_rnn_variants}. For \textit{standard}, we show the equations for a single pixel trajectory. It computes weights based on the pixel embeddings along that trajectory without knowledge of any other trajectories. For \textit{conv}, it uses a $3 \times 3$ convolution kernel instead of the standard matrix multiply to include information from neighboring trajectories. Lastly, for \textit{convGRU}, we design this architecture based on the convGRU architecture \cite{ballas2015delving} which has an explicit memory state to capture longer-term dependencies. For all three variants, the hidden state is $\left \{ \bb{h}_t, \bb{W}_t \right\}$. However, in the RNN we propagate $\frac{\widetilde{\bb{h}}_{t}}{\widetilde{\bb{W}}_{t}}$, which is the intermediate weighted sum at time $t$. This allows the network to use knowledge of the previous weights and pixel embeddings to calculate $\bb{w}_{t+1}$.

\begin{table*}[t]
\centering
\begin{tabular}{|c|c|c|}
\hline
{\it standard} & {\it conv} & {\it convGRU} \\ \hline
$\bb{c}_t^{i,j} = \textrm{ReLU}\left( W_c \colvec{ \frac{\widetilde{\bb{h}}_{t-1}^{i,j}}{\widetilde{\bb{W}}_{t-1}^{i,j}} & \bb{x}_t^{i,j}} \right)$ & $\bb{c}_t = \textrm{ReLU}\left(W_c * \colvec{\frac{\widetilde{\bb{h}}_{t-1}}{\widetilde{\bb{W}}_{t-1}} & \bb{x}_t}\right)$ & $\bb{z}_t = \sigma \left( W_z * \colvec{\frac{\widetilde{\bb{h}}_{t-1}}{\widetilde{\bb{W}}_{t-1}} & \bb{x}_t} \right)$ \\
$ \bb{w}_t^{i,j} = \sigma\left( W_w \bb{c}_t^{i,j} \right) $ & $\bb{w}_t = \sigma\left(W_w * \bb{c}_t \right)$ & $\bb{r}_t = \sigma\left( W_r * \colvec{\frac{\widetilde{\bb{h}}_{t-1}}{\widetilde{\bb{W}}_{t-1}} & \bb{x}_t} \right)$ \\ 
 & & $ \hat{\bb{c}}_t = \textrm{ReLU}\left( W_{\hat{c}} * \colvec{\bb{r}_t \odot \frac{\widetilde{\bb{h}}_{t-1}}{\widetilde{\bb{W}}_{t-1}} & \bb{x}_t} \right) $ \\
 & & $\bb{c}_t = (1 - \bb{z}_t) \odot \widetilde{\bb{c}}_{t-1} + \bb{z}_t \odot \hat{\bb{c}}_t $ \\
 & & $ \bb{w}_t = \sigma\left( W_w * \bb{c}_t \right) $\\
\hline
\multicolumn{3}{|c|}{$\bb{h}_t = \widetilde{\bb{h}}_{t-1} + \bb{w}_t \odot \bb{x}_t$} \\
\multicolumn{3}{|c|}{$ \bb{W}_t = \widetilde{\bb{W}}_{t-1} + \bb{w}_t $} \\ \hline
\end{tabular}
\caption{PT-RNN variants. For {\it standard}, we show the equations for pixel $(i,j)$, while for the others we show equations in terms of the entire $H \times W \times C$ feature map. Note that for {\it standard}, $W_c \in \R^{1 \times 2C}, W_w \in \R^{1 \times C}$, while for {\it conv} and {\it convGRU}, $W_c, W_w, W_z, W_r, W_{\hat{c}}$ are $3\times 3$ convolution kernels. $*$ denotes convolution and $\sigma$ is the sigmoid nonlinearity.}
\label{table:pt_rnn_variants}
\end{table*}

\section{Proof of Proposition 1}

We note the the following:
\begin{align*}
    \argmin_{\|\bb{w}\|_2 = 1} \frac1n \sumi{i}{n} d(\bb{w}, \bb{y}_i) &= \argmin_{\|\bb{w}\|_2 = 1}\ \frac{1}{2n} \sumi{i}{n} (1 - \bb{w}^\T\bb{y}_i) \\
    &= \argmin_{\|\bb{w}\|_2 = 1}\ \left[1 - \frac1n \sumi{i}{n} \bb{w}^\T \bb{y}_i\right] \\
    &= \argmax_{\|\bb{w}\|_2 = 1}\ \sumi{i}{n} \bb{w}^\T\bb{y}_i \\
    &= \argmax_{\|\bb{w}\|_2 = 1}\ \bb{w}^\T \sumi{i}{n} \bb{y}_i
\end{align*}
Note that the unit vector that maximizes the inner product with a given vector $\bb{v}$ is simply the normalized version of $\bb{v}$ (if $\bb{v} \neq 0$). Thus, the solution to the above problem is $\frac{\sumi{i}{n}\bb{y}_i}{\left \| \sumi{i}{n}\bb{y}_i\right \|_2}$.

\removed{
We first note the the following:
\begin{align*}
    \argmin_{\|\bb{w}\|_2 = 1} \frac1n \sumi{i}{n} d(\bb{w}, \bb{y}_i) &= \argmin_{\|\bb{w}\|_2^2 = 1} \frac{1}{2n} \sumi{i}{n} (1 - \bb{w}^\T\bb{y}_i) \\
    &= \argmin_{\|\bb{w}\|_2^2 = 1} \left[1 - \frac1n \sumi{i}{n} \bb{w}^\T \bb{y}_i\right] \\
    &= \argmax_{\|\bb{w}\|_2^2 = 1} \sumi{i}{n} \bb{w}^\T\bb{y}_i
\end{align*}
where the first inequality uses the fact that the constraints $\|w\|_2 = 1$ and $\|w\|_2^2 = 1$ are equivalent. Note that this problem looks to find the unit vector that maximizes the average inner product with all $\bb{y}_i$. Next, we relax the problem to 
\begin{equation} \label{eq:relaxed_problem}
    \argmax_{\|\bb{w}\|_2^2 \leq 1} \sumi{i}{n} \bb{w}^\T \bb{y}_i
\end{equation}
If Eq. \eqref{eq:relaxed_problem} gives a solution that satisfies the original constraint, then this solution must a the solution to the original problem. Indeed, we show that this is the case. 

Note that Eq. \eqref{eq:relaxed_problem} is a convex problem and that there exists a feasible solution (e.g. $\bb{w} = 0$), thus Slater's condition holds \cite{boyd2004convex}. This means that the primal formulation and dual formulation of Eq. \eqref{eq:relaxed_problem} provide the same solution. Thus, we consider the dual formulation of the problem. We negate Eq. \eqref{eq:relaxed_problem} to turn it back to a minimization problem and look at the Lagrangian:
\begin{equation} \label{eq:lagrangian}
    \mathcal{L}(\bb{w}, \lambda) = - \sumi{i}{n} \bb{w}^\T\bb{y}_i + \lambda \left( \|\bb{w}\|_2^2 - 1 \right)
\end{equation}
To get the dual function, we minimize Eq. \eqref{eq:lagrangian} with respect to $\bb{w}$ by taking the gradient:
\begin{equation}
    \frac{\partial}{\partial \bb{w}} \mathcal{L}(\bb{w}, \lambda) = -\sumi{i}{n} \bb{y}_i + 2\lambda\bb{w}
\end{equation}
Setting this to 0 gives us
\begin{equation} \label{eq:w_star}
    \bb{w}^* = \frac{1}{2\lambda}\sumi{i}{n}\bb{y}_i
\end{equation}
We define $S_n = \sumi{i}{n} \bb{y}_i$, and plug the above back into Eq. \eqref{eq:lagrangian} to give:
\begin{align}
    g(\lambda) &= - \frac{1}{2\lambda} \left \| S_n \right \|_2^2 + \frac{1}{4\lambda} \left \| S_n \right \|_2^2 - \lambda \\
    &= -\frac{1}{4\lambda} \left \| S_n \right \|_2^2 - \lambda
\end{align}
Thus, the dual problem is:
\begin{equation} \label{eq:dual_problem}
    \max_{\lambda \geq 0}\ -\frac{1}{4\lambda} \left \| S_n \right \|_2^2 - \lambda
\end{equation}
To solve the dual, we take the gradient
\begin{equation}
    \frac{\partial}{\partial \lambda} g(\lambda) = \frac{1}{4\lambda^2} \left \| S_n \right\|_2^2 - 1
\end{equation}
Setting this to 0 gives
\begin{equation}
    \lambda^* = \frac12 \left \|S_n \right\|_2
\end{equation}
Note that since $\lambda^* \geq 0$, this satisfies the constraints in Eq. \eqref{eq:dual_problem}, thus is the solution. Plugging this back into Eq. \eqref{eq:w_star} gives
\begin{equation}
    \bb{w}^* = \frac{S_n}{\left \| S_n \right\|_2} = \frac{\sumi{i}{n} \bb{y}_i}{\left \| \sumi{i}{n} \bb{y}_i \right \|_2}
\end{equation}
}

\section{Dataset Details}
\paragraph{FT3D} The Flying Things 3D dataset (FT3D) \cite{MIFDB16} is a synthetic dataset comprised of approximately 2250 training and 450 test videos of 10 images each. Each video is created by instantiating a background with static objects and populating the scene by having sampled foreground objects from ShapeNet \cite{shapenet2015} flying along randomized 3D trajectories. Segmentation masks of all objects (foreground and background) are provided. While \cite{MIFDB16} does not provide information about which objects are foreground, \cite{tokmakov2017mpnet} provided foreground labels by identifying the objects which underwent changes in 3D coordinates. We combined this with the object segmentation masks to produce foreground motion clustering masks. We use this dataset for both evaluation and pre-training. Performance on this dataset is measured by intersection over union (IoU) of the foreground masks. 

\paragraph{DAVIS} The DAVIS2016 dataset \cite{Perazzi2016} is a collection of 50 videos of approximately 3500 images, split into a 30 training videos and 20 test videos. Each video is accompanied by pixel-dense foreground labels at each frame. We evaluate on the test set for video foreground segmentation only. The DAVIS2017 dataset \cite{Pont-Tuset_arXiv_2017} expands on DAVIS2016 and provides 90 publicly available video sequences with full pixel-dense annotation. DAVIS2017 focuses on semi-supervised video segmentation (as opposed to unsupervised, i.e. foreground segmentation) and provides multiple labels per video. However, not every object labeled is foreground, and not every foreground object is labeled, thus this dataset is not suitable for the task of object discovery. Despite this, we leverage the sequences for training. We use the $\mathcal{J}$-measure (IoU) and the $\mathcal{F}$-measure as defined by \cite{Perazzi2016} as evaluation metrics for DAVIS2016.

\paragraph{FBMS} The Freiburg-Berkeley motion segmentation dataset \cite{ochs2014segmentation} consists of 59 videos split into 29 training videos and 30 test videos. The videos can be up to 800 images long, and approximately every 20th frame has ground truth motion segmentation labels. The inconsistency and ambiguity in motion segmentation dataset labels inspired \cite{bideau2016rubric} to rigorously define the problem of motion segmentation and provide corrected labels which we use in this work. \removed{Our problem of object discovery is essentially what \cite{bideau2016rubric} describe as tracking by motion analysis. However, their problem definition is similar to ours, thus we can fairly train and evaluate using these corrected labels.} Performance on this dataset is measured by precision, recall, F-score, and $\Delta$Obj as described in \cite{ochs2014segmentation, bideau2018best}. 

\paragraph{Others} We also show results on the Complex Background \cite{narayana2013coherent} and Camouflaged Animal \cite{bideau2016s} datasets. These datasets are small and contain 5 and 9 sequences, respectively. Labels are corrected and provided by \cite{bideau2016rubric}. We use the same metrics for evaluation as the FBMS dataset.

\section{DAVIS-m}

We hand-select 42 videos from the DAVIS2017 \cite{Pont-Tuset_arXiv_2017} train and val datasets (90 videos total) that roughly satisfy the rubric of \cite{bideau2016rubric}. We denote this dataset as DAVIS-m, and use it to supplement the small training dataset of FBMS (29 videos). In hand-selecting these videos, we make sure that only (and all of) the foreground objects are labeled, and that the foreground objects are correctly separated into different objects. For example, the video \textit{classic-car} shows two people in a car with a segmentation mask for the car, and separate segmentation masks for the people. This is incredibly difficult for an algorithm to properly segment using motion cues (and does not fit the rubric of \cite{bideau2016rubric}), thus is not included in DAVIS-m. The exact videos are given in Table \ref{table:davis_m}, where we show all 42 videos. There are 27 videos that have a single object (i.e. video foreground segmentation) and 15 videos with multiple objects.

\begin{table}[]
    \centering
    \begin{tabular}{|c|c|}
        \hline
        Multi-object & Foreground \\ \hline
        \textit{boxing-fisheye} & \textit{bear} \\
        \textit{cat-girl} & \textit{bike-packing} \\
        \textit{disc-jockey} & \textit{blackswan} \\
        \textit{dog-gooses} & \textit{breakdance-flare} \\
        \textit{dogs-jump} & \textit{bus} \\
        \textit{gold-fish} & \textit{car-shadow} \\
        \textit{judo} & \textit{car-turn} \\
        \textit{kid-football} & \textit{cows} \\
        \textit{loading} & \textit{dance-twirl} \\
        \textit{night-race} & \textit{dog} \\
        \textit{pigs} & \textit{drift-chicane} \\
        \textit{planes-water} & \textit{drift-straight} \\
        \textit{sheep} & \textit{drift-turn} \\
        \textit{tuk-tuk} & \textit{elephant} \\
        \textit{walking} & \textit{flamingo} \\
         & \textit{goat} \\
         & \textit{hike} \\
         & \textit{koala} \\
         & \textit{libby} \\
         & \textit{lucia} \\
         & \textit{mallard-fly} \\
         & \textit{mallard-water} \\
         & \textit{parkour} \\
         & \textit{rallye} \\
         & \textit{rhino} \\
         & \textit{rollerblade} \\
         & \textit{soccerball} \\
        \hline
    \end{tabular}
    \caption{DAVIS-m videos. The left column shows the 15 multi-object videos (2 or more objects), and the right column shows the 27 single-object videos (i.e. video foreground segmentation).}
    \label{table:davis_m}
\end{table}

\section{Object Discovery results on FT3D}

To facilitate motion segmentation and object discovery research, we provide our motion segmentation results for the FT3D \cite{MIFDB16} testset. We provide numbers for the metrics described in \cite{ochs2014segmentation, bideau2018best}, namely precision, recall, F-score, and $\Delta$Obj for the multi-object and foreground settings. We trained our full model for 150k iterations using the motion segmentation labels we extracted from foreground labels \cite{tokmakov2017mpnet} and object segmentation labels \cite{MIFDB16}. The results are provided in Table \ref{table:FT3D_results}.

\begin{table}[]
    \centering
    \begin{tabular}{|cccc|ccc|}
    \hline
        \multicolumn{4}{|c|}{Multi-object} & \multicolumn{3}{c|}{Foreground} \\ \hline
        \textcolor{orange}{P} & \textcolor{cyan}{R} & \textcolor{purple}{F} & $\Delta$Obj & \textcolor{orange}{P} & \textcolor{cyan}{R} & \textcolor{purple}{F} \\ \hline
        74.3 & 75.1 & 72.9 & 2.46  & 96.4 & 97.7 & 96.9  \\ \hline
    \end{tabular}
    \caption{Results on FT3D}
    \label{table:FT3D_results}
\end{table}

\section{About the name ``Object Discovery''}

Our definition of object discovery is motivated by the robotic application of discovering objects via their motion. Our definition of object discovery is almost identical to that of (multi-object) ``motion segmentation'' as defined in \cite{bideau2016rubric}, except that objects should be tracked even when there is no observed flow at certain frames.
